# Supplementary material for: FM-EAC: Feature Model-based Enhanced Actor-Critic for Multi-Task Control in Dynamic Environments
Source: arXiv:2512.15430 source file (2025-12-17)
Supplement: Supplementary file 1 [file Appendix.tex]

\section{Appendices}
\appendix

\subsection{Explanation of Demonstration Code}
\label{demo_code}

The demonstration code can be downloaded from \href{https://anonymous.4open.science/r/Mobisys_PAN-GNN-370D/}{link to demonstration code}.
In the demonstration code, there are six files. ``ReadMe.md" explains the code in general. \\
``Folder\_structure" shows the architecture of the entire code, which will be released upon acceptance. The other four files are the demonstration code detalied below.

% \vspace{1.5em}

\subsubsection{General Description}
For anonymity, information regarding city, terrain, and document paths has been omitted. 
% Additionally, all comments have been removed to improve clarity.
To facilitate understanding of the proposed algorithms, only agent-related code segments are presented here. The complete folder structure is documented in the accompanying ``Folder\_structure.pdf".
Following acceptance, we will release the full executable code for function validation.

% \vspace{1.5em}

% \textit{Code Modules Overview}:
The demonstration code includes the following four files.

\textit{agri\_eac\_gnn\_model.py}: Implements network architectures for GNN, BPN, and FM-EAC tailored to agricultural applications.

\textit{agri\_eac\_pan\_model.py}: Implements network architectures for PAN, BPN, and FM-EAC tailored to agricultural applications.
    
\textit{urban\_eac\_gnn\_model.py}: Implements network architectures for GNN and FM-EAC tailored to urban applications.
    
\textit{urban\_eac\_pan\_model.py}: Implements network architectures for PAN and FM-EAC tailored to urban applications.

% \vspace{1.5em}

\subsubsection{Detailed Description of Key Modules}
The explanation of key modules (i.e., elements and functions) in each file is detailed as follows.

% \vspace{1.5em}
\textit{agri\_eac\_gnn\_model.py}:
\begin{itemize}
    \item Actor: Policy network generating actions conditioned on input states.
    \item Critic: Evaluation network estimating Q-values for state-action pairs.
    \item BatteryPredictionNetwork: Predicts energy consumption based on state and environmental features.
    \item normalize\_adjacency\_matrix(A): Normalizes adjacency matrices used in graph convolution layers.
    \item GCNLayer: Single graph convolutional layer processing node features with normalized adjacency.
    \item GNN: Two-layer graph neural network producing a global graph representation via node features and adjacency.
    \item GNN\_Agent:
    \item compute\_gnn\_loss(batch\_state, batch\_action, batch\_reward, batch\_done): Computes critic loss for training GNN and critic networks.
    \item choose\_action(state, explore=True): Selects an action given the current state, optionally with exploration noise.
    \item store\_transition(state, action, reward, next\_state, done): Saves experience tuples into replay buffer, managing buffer capacity.
    \item update(): Samples batches from replay buffer and updates GNN, Critic, and Actor networks with soft target updates.
    \item save(i, path, eps): Saves model weights (Actor, Critics, GNN) to checkpoint files.
    \item load(i, path, eps): Loads model weights from checkpoint files; raises error if files are absent.
\end{itemize}

% \vspace{1.5em}

\textit{agri\_eac\_pan\_model.py}:
\begin{itemize}
    \item Actor: Policy network generating actions based on input states.
    \item Critic: Value network estimating Q-values for state-action pairs.
    \item BatteryPredictionNetwork: Estimates energy consumption from input state and environment features.
    \item PointArrayFeatureExtractor: Extracts features from input environmental point array data.
    \item PAN\_Agent:
    \item choose\_action(state, explore=True): Selects action given state, optionally applying exploration noise.
    \item store\_transition(state, action, reward, next\_state, done): Stores experience tuples in replay buffer, handling buffer size constraints.
    \item update(): Samples from replay buffer and updates Critic and Actor networks, including soft target network updates.
    \item save(i, path, eps): Persists model parameters (Actor, Critics) to disk with iteration and episode identifiers.
    \item load(i, path, eps): Loads model parameters from saved checkpoints; raises error if missing.
\end{itemize}

% \vspace{1.5em}

\textit{urban\_eac\_gnn\_model.py}:
\begin{itemize}
    \item Actor: Policy network producing two types of actions from input states:
    \item Primary action (mean mu and standard deviation std): continuous actions modeled as a Gaussian distribution.
    \item Secondary action (softmax\_out): categorical distribution over three discrete options via softmax.
    \item Critic\_Pri: Value network estimating Q-values for state-primary action pairs.
    \item Critic\_Sec: Value network estimating Q-values for state-secondary action pairs.
    \item normalize\_adjacency\_matrix(A): Adds self-loops and normalizes adjacency matrix for graph convolutional layers.
    \item GCNLayer: Single graph convolution layer performing adjacency normalization and learnable feature transformation.
    \item GNN: Two-layer graph neural network processing node features and adjacency, outputting global graph features by mean pooling.
    \item GNN\_Agent:
    \item compute\_gnn\_loss(batch\_state, batch\_action): Computes loss on critic Q-values to update the GNN network by encouraging higher Q-values.
    \item update(): Conducts a training step by sampling batches, computing target Q-values, updating critics and actors, and applying GNN loss optimization.
    \item choose\_action(state): Samples actions combining continuous primary actions and discrete secondary actions from the actor output.
    \item save(i, path, eps): Saves model weights (actor, critics, GNN) to checkpoint files.
    \item load(i, path, eps): Loads model weights from checkpoint files.

\end{itemize}

% \vspace{1.5em}

\textit{urban\_eac\_pan\_model.py}:
\begin{itemize}
    \item Actor: Policy network outputting two action types from the input state:
    \item Primary action (mean mu and standard deviation std): continuous actions modeled as a Gaussian distribution, dimension (action\_dim - 3).
    \item Secondary action (softmax\_out): categorical distribution over three discrete options via softmax.
    \item Critic\_Pri: Value network estimating Q-values for state and primary action pairs (continuous).
    \item Critic\_Sec: Value network estimating Q-values for state and secondary action pairs (discrete, one-hot encoded).
    \item PointArrayFeatureExtractor: Extracts features from environmental point array inputs.
    \item PAN\_Agent:
    \item update(): Executes a training iteration by sampling from replay buffer, computing target Q-values, optimizing critics via MSE loss, and updating actor networks to maximize expected Q-values.
    \item choose\_action(state): Samples combined continuous and discrete actions from actor outputs.
    \item save(i, path, eps): Saves current model parameters (actor and critics) with iteration and episode labels.
    \item load(i, path, eps): Loads model parameters from saved checkpoints.
\end{itemize}

\subsection{Environmental Parameter and Hyperparameter Settings}
\begin{table*}[t]
\caption{Environmental Parameters for the Urban Application.}
\label{env_urban}
\centering
\begin{tabular}{ |c|c|c|c|c|c|c|c|} \hline
\textbf{Symbol} & \textbf{Definition} & \textbf{Value} &  \textbf{Unit} & \textbf{Symbol} & \textbf{Definition} & \textbf{Value} &  \textbf{Unit} \\
\hline
$pu_{x-\text{min}}$ & Task Space Left Edge & $0$ & m &$pu_{x-\text{max}}$ & Task Space Right Edge & $800$ & m\\
$pu_{y-\text{min}}$ & Task Space Back Edge & $0$ & m &$pu_{y-\text{max}}$ & Task Space Front Edge & $800$ & m\\
$pu_{z-\text{min}}$ & Task Space Bottom Edge & $180$ & m &$pu_{z-\text{max}}$ & Task Space Top Edge & $220$ & m\\
$d_{\text{end}}$ & Advance End Task Distance& 50 &m &$V_{x-\text{max}}$ & $x$ Dire. Maximum Velocity & 8 & $\text{m/s}$\\
$V_{y-\text{max}}$ & $y$ Dire. Maximum Velocity & 8 & $\text{m/s}$ &$V_{z-\text{max}}$ &$z$ Dire. Maximum Velocity & 8 & $\text{m/s}$\\
$T_\text{end}$ & Maximum Mission Time& 100 &s & $n_\text{UAV}$ & UAV Number& $2-6$&-\\
$n_{\text{BS}}$ & BS Number & $3,4$ &- & $n_{\text{IoT}}$ & IoT Device Number & $[0,100]$& -\\
$\epsilon$ & Allocation Proportion & 0.8 &- & $BC$ & Battery Capacity& $155520$& $\text{J}$\\
$Pw_{\text{cmp}}$ & Computation Power& 20& W &$ pw_{\text{ut}}$& UAV Transmission Power & 20 & dBm\\ 
$Pw_{ur}$ & UAV Received Power & 20 & dBm & $m_{\text{UAV}}$ & UAV Mass & 0.2 &kg \\
$g$ & Gravitational Acceleration & 9.8&- & $\rho_{\text{air}}$ & Air Density & 1.225 & $\text{kg/m}^3$\\
$v_{\text{th}}$& Hovering Speed Threshold & 0.1 &$\text{m/s}$ & $C_d$ & Viscosity Coefficient& 0.5 & $-$\\
$n_{\text{prp}}$ &Propeller Number & 4 &- & $R_{\text{prp}}$& Propeller Radius& 0.1 & m\\
$\eta$ &Mechanical Efficiency & 0.8 & - & $A_{\text{surf}}$& UAV Fuselage Area & 0.01 & $\text{m}^2$\\
$m_{\text{ULA}}$& ULA Horizontal Dimension& 8&- &$n_{\text{ULA}}$& ULA Vertical Dimension& 8&-\\
$d_{\text{ULA}}$ & Element Distance & 0.05& m &$\theta_{\text{main}}$ & Horizontal Main Lobe Dire. & 0 & $^\circ$\\
$\phi{\text{main}}$ & Vertical Main Lobe Dire. & 80& $^\circ$ & $c$ & Light Speed & 3e8& $\text{m/s}$\\
$\Theta_{3\text{dB}}$ & Horizontal 3dB Beam-width & 65 & $^\circ$ & $\Phi_{3\text{dB}}$ & Vertical 3dB Beam-width&65&$^\circ$ \\
$G_{\text{element}}$ & Antenna Element Gain & 5 &dB & $k_B$ &  Boltzmann Constant&1.38e-23&-\\
$T_K$ &Temperature in Kelvin& 298 & K& $Bw$ & Bandwidth & 20 &MHz \\
$f_{BS}$ & BS Frequency & 3.5 & GHz &$f_{IoT}$ & IoT Device Frequency & 5.9 & GHz \\
$m$ & Up-link Limitation & 3 & -& $k_{\text{end}}$ & Discretized End Time & 100 & -\\
\hline
\end{tabular}
\end{table*}

\begin{table*}[t]
\caption{Hyperparameters for the urban application.}
\label{hyper_urban}
\centering
\begin{tabular}{ |c|c|c|c|c|c|} \hline
\textbf{Symbol} & \textbf{Definition} & \textbf{Value}  & \textbf{Symbol} & \textbf{Definition} & \textbf{Value} \\
\hline
$\alpha_1$ & Weight Parameter for Length &1&$\alpha_2$ & Weight Parameter for Flight Height &0.75\\
$\alpha_3$ & Weight Parameter for SINR &2.5&$\alpha_4$ & Weight Parameter for Energy Consumption &0.1\\
$\alpha_5$ & Weight Parameter for QoS  &0.75&$\alpha_6$ & Weight Parameter for Out and Collision &10\\$\alpha_7$& Weight parameter for safety risk & 0.1 & $\alpha_8$& Partial Reward Weight & 10 \\$\gamma$ & Discounted Factor& 0.99 & $\mathcal{HN}$ & Normal Hidden Layers & 3\\
$r_a$ & Learning Rate for Actor& $10^{-5}$ &$r_{ct}$ & Learning Rate for Total Reward Critic& $10^{-4}$\\
$r_{cp}$ & Learning Rate for Partial Critic & $10^{-5}$&$\mathcal{B_P}$ & PAN Training Batch Size & $512$\\
$\mathcal{D}$ & Replay Buffer Size & $2^{16}$&$\mathcal{B}$ &RL Training Batch Size & 256\\
$epi_{\text{max}}$ & Maximum Training Episode & 1000 & $epo_{\text{max}}$ &PAN Pre-training Maximum Epoch &100\\
$\xi$ & Soft Update parameter & 0.01 & $k_{\text{max}}$ & Maximum Timestep& 100\\
$r_G$ & Learning Rate for GNN & $10^{-3}$ &$r_P$ & Learning Rate for PAN & $10^{-4}$\\
$\tilde{S}$ & Scenario Number &3 &$\tilde{X}$ & PMP Trace Number & 30\\

$\beta_P$ & PAN Normalization Coefficient & 0.01& $\beta_G$ & GNN Normalization Coefficient & 0.01\\
\hline
\end{tabular}
\end{table*}

\begin{table*}[t]
\caption{Environmental Parameters for the Agricultural Application.}
\label{env_agri}
\centering
\begin{tabular}{ |c|c|c|c|c|c|c|c|} \hline
\textbf{Symbol} & \textbf{Definition} & \textbf{Value} &  \textbf{Unit} & \textbf{Symbol} & \textbf{Definition} & \textbf{Value} &  \textbf{Unit} \\
\hline
$pu_{x-\text{min}}$ & Task Space Left Edge & $0$ & m &$pu_{x-\text{max}}$ & Task Space Right Edge & $400$ & m\\
$pu_{y-\text{min}}$ & Task Space Back Edge & $0$ & m &$pu_{y-\text{max}}$ & Task Space Front Edge & $400$ & m\\
$pu_{z-\text{min}}$ & Task Space Bottom Edge & $30$ & m &$pu_{z-\text{max}}$ & Task Space Top Edge & $150$ & m\\
$d_{\text{end}}$ & Advance End RTH Distance& 30 &m &$V_{x-\text{max}}$ & $x$ Dire. Maximum Velocity& 10 & $\text{m/s}$\\
$V_{y-\text{max}}$ & $y$ Dire. Maximum Velocity & 10 & $\text{m/s}$ &$V_{z-\text{max}}$ &$z$ Dire. Maximum Velocity & 5 & $\text{m/s}$\\
$T_{f_{\text{end}}}$ & Maximum COL Time& 500 &s &$T_{r_{\text{end}}}$ & Maximum RTH Time& 100 &s\\  
$n_\text{UAV}$ & UAV Number& $4$&-& $n_{\text{WS}}$ & WS Number & $400$& -\\
$\text{AoI}_{\text{max}}$ & Maximum AoI of WSs & 0.8 &- & $BC$ & Battery Capacity& $155520$& $\text{J}$\\
$Pw_{\text{cmp}}$ & Computation Power& 20& W & $T_{\text{update}_{\text{AoI}}}$& AoI Updating Time & 40,50,60& s\\ 
$Pw_{ur}$ & UAV Received Power & 30 & dBm & $m_{\text{UAV}}$ & UAV Mass & 0.2 &kg \\
$g$ & Gravitational Acceleration & 9.8&- & $\rho_{\text{air}}$ & Air Density & 1.225 & $\text{kg/m}^3$\\
$v_{\text{th}}$& Hovering Speed Threshold & 0.1 &$\text{m/s}$ & $C_d$ & Viscosity Coefficient& 0.5 & $-$\\
$n_{\text{prp}}$ &Propeller Number & 4 &- & $R_{\text{prp}}$& Propeller Radius& 0.1 & m\\
$\eta$ &Mechanical Efficiency & 0.8 & - & $A_{\text{surf}}$& UAV Fuselage Area & 0.01 & $\text{m}^2$\\
$f_{c}$ & Signal Frequency & 2.8 & GHz &$d_{\text{WS}}$& Distance between WSs & 20 & m\\
\hline
\end{tabular}
\end{table*}

\begin{table*}[t]
\caption{Hyperparameters for the agricultural application.}
\label{hyper_agri}
\centering
\begin{tabular}{ |c|c|c|c|c|c|} \hline
\textbf{Symbol} & \textbf{Definition} & \textbf{Value}  & \textbf{Symbol} & \textbf{Definition} & \textbf{Value} \\
\hline
$\alpha_1$ & AoI Weight Parameter in Collection Task &2&$\alpha_2$ & Penalty for visiting same grids &0.5\\
$\alpha_3$ & AoI Weight Parameter in Return Task &0.1& $\alpha_4$ & Motivation for Exploration &0.01\\
$\alpha_5$ & Weight Parameter for flying out &10&$\gamma$ & Discounted Factor& 0.99 \\
$r_a$ & Learning Rate for Actor& $10^{-4}$ &$r_{ct}$ & Learning Rate for Critic& $10^{-5}$\\
$r_b$ & Learining rate for BPN &$10^{-5}$&$\mathcal{B_P}$ & PAN Training Batch Size & $512$\\
$\mathcal{D}$ & Replay Buffer Size & $2^{16}$&$\mathcal{B}$ &RL Training Batch Size & 128\\
$epi_{\text{max}}$ & Maximum Training Episode & 10000 & $epo_{\text{max}}$ &PAN Pre-training Maximum Epoch &1000\\
$\xi$ & Soft Update parameter & 0.005 &$\tilde{S}$ & Scenario Number &10 \\
$r_G$ & Learning Rate for GNN & $10^{-3}$ &$r_P$ & Learning Rate for PAN & $10^{-4}$\\

$\beta_P$ & PAN Normalization Coefficient & 0.01& $\beta_G$ & GNN Normalization Coefficient & 0.01\\
\hline
\end{tabular}
\end{table*}
